# Supplementary material for: Learning Hidden Dynamics using Intelligent Automatic Differentiation
Source: arXiv:1912.07547 source file (2019-12-16)
Supplement: Supplementary file 1 [file ex_supplement.pdf]

# SUPPLEMENTARY MATERIALS: LEARNING HIDDEN DYNAMICS USING INTELLIGENT AUTOMATIC DIFFERENTIATION[*]

KAILAI XU[†], DONGZHUO LI[‡], ERIC DARVE[§], AND JERRY M. HARRIS[¶]

**SM1. Discrete Adjoint State Methods for FWI.** We derive the adjoint-state equations and the gradient of the misfit function with respect to velocity for example. Starting from the discretization Equation (SM2.4), we obtain the Lagrangian

(SM1.1)

$$
\begin{aligned}
&\mathcal{L}\Big(\varphi_{ij}^{n+\frac12}, \psi_{ij}^{n+\frac12}, p_{ij}^{n+\frac12}, \tilde\varphi_{ij}^{n+1}, \tilde\psi_{ij}^{n+1}, u_{ij}^{n+1}, v_{ij}^{n+1}, K_{ij},\\
&\qquad {}^{\dagger}\varphi_{ij}^{n+\frac12}, {}^{\dagger}\psi_{ij}^{n+\frac12}, {}^{\dagger}p_{ij}^{n+\frac12}, {}^{\dagger}\tilde\varphi_{ij}^{n+1}, {}^{\dagger}\tilde\psi_{ij}^{n+1}, {}^{\dagger}u_{ij}^{n+1}, {}^{\dagger}v_{ij}^{n+1}\Big)\\
&= \frac12\sum_{r=1}^{N_r}(d_r^{n+\frac12} - R_r p_{ij}^{n+\frac12})^2\\
&+ \left\langle {}^{\dagger}\varphi_{ij}^{n+\frac12},\quad \varphi_{ij}^{n+\frac12} - \varphi_{ij}^{n-\frac12}\exp\left(-\alpha_x^i\Delta t\right) - \eta_x^i\left(\frac{\exp\left(-\alpha_x^i\Delta t\right)-1}{\alpha_x^i}\right)\frac{\delta_x u_{ij}^n}{\Delta x}\right\rangle\\
&+ \left\langle {}^{\dagger}\psi_{ij}^{n+\frac12},\quad \psi_{ij}^{n+\frac12} - \psi_{ij}^{n-\frac12}\exp\left(-\alpha_y^j\Delta t\right) - \eta_y^j\left(\frac{\exp\left(-\alpha_y^j\Delta t\right)-1}{\alpha_y^j}\right)\frac{\delta_y v_{ij}^n}{\Delta y}\right\rangle\\
&+ \Bigg\langle {}^{\dagger}p_{ij}^{n+\frac12},\quad p_{ij}^{n+\frac12} - p_{ij}^{n-\frac12} -\\
&\qquad K_{ij}\left(\frac{1}{\kappa_x^i}\frac{\delta_x u_{ij}^n}{\Delta x} + \varphi_{ij}^{n+\frac12} + \frac{1}{\kappa_y^j}\frac{\delta_y v_{ij}^n}{\Delta y} + \psi_{ij}^{n+\frac12}\right)\Delta t - s_{ij}^n\Delta t\Bigg\rangle\\
&+ \left\langle {}^{\dagger}\tilde\varphi_{ij}^{n+1},\quad \tilde\varphi_{ij}^{n+1} - \tilde\varphi_{ij}^{n}\exp\left(-\tilde\alpha_x^i\Delta t\right) - \tilde\eta_x^i\left(\frac{\exp\left(-\tilde\alpha_x^i\Delta t\right)-1}{\tilde\alpha_x^i}\right)\frac{\delta_x p_{i,j+\frac12}^{n+\frac12}}{\Delta x}\right\rangle\\
&+ \left\langle {}^{\dagger}\tilde\psi_{ij}^{n+1},\quad \tilde\psi_{ij}^{n+1} - \tilde\psi_{ij}^{n}\exp\left(-\tilde\alpha_y^j\Delta t\right) - \tilde\eta_y^j\left(\frac{\exp\left(-\tilde\alpha_y^j\Delta t\right)-1}{\tilde\alpha_y^j}\right)\frac{\delta_y p_{i+\frac12,j}^{n+\frac12}}{\Delta y}\right\rangle\\
&+ \left\langle {}^{\dagger}u_{ij}^{n+1},\quad u_{ij}^{n+1} - u_{ij}^n - \frac{1}{\rho_{ij}}\left(\frac{1}{\kappa_x^i}\frac{\delta_x p_{i,j+\frac12}^{n+\frac12}}{\Delta x} + \tilde\varphi_{ij}^{n+1}\right)\Delta t\right\rangle\\
&+ \left\langle {}^{\dagger}v_{ij}^{n+1},\quad v_{ij}^{n+1} - v_{ij}^n - \frac{1}{\rho_{ij}}\left(\frac{1}{\kappa_y^j}\frac{\delta_y p_{i+\frac12,j}^{n+\frac12}}{\Delta y} + \tilde\psi_{ij}^{n+1}\right)\Delta t\right\rangle,
\end{aligned}
$$

[*]Kailai Xu and Dongzhuo Li contributed equally to this paper.
[†]Institute for Computational and Mathematical Engineering, Stanford University, Stanford, CA, 94305 (kailaix@stanford.edu)
[‡]Department of Geophysics, Stanford University, Stanford, CA, 94305 (lidongzh@stanford.edu)
[§]Mechanical Engineering and Institute for Computational and Mathematical Engineering, Stanford University, Stanford, CA, 94305 (darve@stanford.edu)
[¶]Department of Geophysics and Institute for Computational and Mathematical Engineering, Stanford University, Stanford, CA, 94305 (harrisgp@stanford.edu)



*This manuscript is for review purposes only.*

where quantities with the dagger are corresponding Lagrange multipliers or adjoint-state variables, operator $R_r$ is the restriction onto the position of receivers, and the angle brackets denote summation over spatial indices $ij$ and the temporal index $n$. According to the KKT condition, taking the derivative of $\mathcal{L}$ with respect to normal variables and setting them to zero, we arrive at the adjoint equations:

(SM1.2)

$$\begin{aligned}
\frac{{}^\dagger v_{ij}^n - {}^\dagger v_{ij}^{n+1}}{\Delta t} &= -\eta_y^j \left(\frac{\exp\left(-\alpha_y^i \Delta t\right) - 1}{\alpha_y^i}\right) \frac{{}^\dagger \psi_{ij}^{n+\frac{1}{2}}}{\Delta y \Delta t} - \frac{K_{ij}}{\kappa_y^j} \frac{\delta_y\, {}^\dagger p_{ij}^{n+\frac{1}{2}}}{\Delta y} \\
\frac{{}^\dagger u_{ij}^n - {}^\dagger u_{ij}^{n+1}}{\Delta t} &= -\eta_x^i \left(\frac{\exp\left(-\alpha_x^i \Delta t\right) - 1}{\alpha_x^i}\right) \frac{{}^\dagger \varphi_{ij}^{n}}{\Delta x \Delta t} - \frac{K_{ij}}{\kappa_x^i} \frac{\delta_x\, {}^\dagger p_{ij}^{n+\frac{1}{2}}}{\Delta x} \\
{}^\dagger \tilde{\psi}_{ij}^n &= {}^\dagger \tilde{\psi}_{ij}^{n+1} \left(-\tilde{\alpha}_y^j \Delta t\right) + \frac{1}{\rho_{ij}} {}^\dagger \tilde{v}_{ij}^n \Delta t \\
{}^\dagger \tilde{\varphi}_{ij}^n &= {}^\dagger \tilde{\varphi}_{ij}^{n+1} \left(-\tilde{\alpha}_x^i \Delta t\right) + \frac{1}{\rho_{ij}} {}^\dagger \tilde{u}_{ij}^n \Delta t \\
\frac{{}^\dagger p_{ij}^{n-\frac{1}{2}} - {}^\dagger p_{ij}^{n+\frac{1}{2}}}{\Delta t} &= -\tilde{\eta}_x^i \left(\frac{\exp\left(-\tilde{\alpha}_x^i \Delta t\right) - 1}{\tilde{\alpha}_x^i}\right) \frac{\delta_x\, {}^\dagger \tilde{\varphi}_{ij}^n}{\Delta x \Delta t} \\
&\quad - \tilde{\eta}_y^j \left(\frac{\exp\left(-\tilde{\alpha}_y^j \Delta t\right) - 1}{\tilde{\alpha}_y^j}\right) \frac{\delta_y\, {}^\dagger \tilde{\psi}_{ij}^n}{\Delta y \Delta t} \\
&\quad - \frac{1}{\rho_{ij} \kappa_x^i} \frac{\delta_x\, {}^\dagger u_{ij}^n}{\Delta x} - \frac{1}{\rho_{ij} \kappa_y^j} \frac{\delta_x\, {}^\dagger v_{ij}^n}{\Delta y} + \sum_{r=1}^{N_r} R_r^T \left(d_r^{n-\frac{1}{2}} - R_r^T p_{ij}^{n-\frac{1}{2}}\right) \frac{1}{\Delta t} \\
{}^\dagger \psi_{ij}^{n-\frac{1}{2}} &= {}^\dagger \psi_{ij}^{n+\frac{1}{2}} \exp\left(-\alpha_y^j \Delta t\right) + K_{ij}\, {}^\dagger p_{ij}^{n-\frac{1}{2}} \Delta t \\
{}^\dagger \varphi_{ij}^{n-\frac{1}{2}} &= {}^\dagger \varphi_{ij}^{n+\frac{1}{2}} \exp\left(-\alpha_x^j \Delta t\right) + K_{ij}\, {}^\dagger p_{ij}^{n-\frac{1}{2}} \Delta t.
\end{aligned}$$

Note that at the final time step $N_t$, the adjoint equations are

(SM1.3)

$$\begin{aligned}
&{}^\dagger v_{ij}^{N_t} = 0, \qquad {}^\dagger u_{ij}^{N_t} = 0, \qquad {}^\dagger \tilde{\psi}_{ij}^{N_t} = \frac{1}{\rho_{ij}} {}^\dagger \tilde{v}_{ij}^{N_t} \Delta t = 0, \qquad {}^\dagger \tilde{\varphi}_{ij}^{N_t} = \frac{1}{\rho_{ij}} {}^\dagger \tilde{u}_{ij}^{N_t} \Delta t = 0 \\
&{}^\dagger p_{ij}^{N_t - \frac{1}{2}} = \sum_{r=1}^{N_r} R_r^T \left(d_r^{N_t - \frac{1}{2}} - R_r^T p_{ij}^{N_t - \frac{1}{2}}\right) \\
&{}^\dagger \psi_{ij}^{N_t - \frac{1}{2}} = K_{ij}\, {}^\dagger p_{ij}^{N_t - \frac{1}{2}} \Delta t \\
&{}^\dagger \varphi_{ij}^{N_t - \frac{1}{2}} = K_{ij}\, {}^\dagger p_{ij}^{N_t - \frac{1}{2}} \Delta t.
\end{aligned}$$

Similarly, taking the derivative of $\mathcal{L}$ with respect to model parameter $K_{ij}$, we get the gradient of the misfit function with respect to $K_{ij}$ as

(SM1.4)

$$\begin{aligned}
\nabla_{K_{ij}} J &= -\sum_{n=1}^{N_t} \left( {}^\dagger p_{ij}^{n+\frac{1}{2}} \left( \frac{1}{\kappa_x^i} \frac{\delta_x u_{ij}^n}{\Delta x} + \varphi_{ij}^{n+\frac{1}{2}} + \frac{1}{\kappa_y^j} \frac{\delta_y v_{ij}^n}{\Delta y} + \psi_{ij}^{n+\frac{1}{2}} \right) \Delta t \right) \\
&= -\sum_{n=1}^{N_t} \left( {}^\dagger p_{ij}^{n+\frac{1}{2}} \frac{p_{ij}^{n+\frac{1}{2}} - p_{ij}^{n-\frac{1}{2}} - s_{ij}^n \Delta t}{K_{ij}} \right).
\end{aligned}$$

Therefore, the gradient with respect to wave velocity is

$$\nabla_{c_{ij}} J = 2c_{ij}\rho_{ij}\nabla_K J = -\frac{2}{c_{ij}}\sum_{n=1}^{N_t}\left({}^{\dagger}p_{ij}^{n+\frac{1}{2}}\left(p_{ij}^{n+\frac{1}{2}} - p_{ij}^{n-\frac{1}{2}} - s_{ij}^{n}\Delta t\right)\right). \tag{SM1.5}$$

The procedures we are performing here are exactly equivalent to the reverse mode automatic differentiation.

## SM2. Discretization of the Wave Equation with the CPML Boundary Condition.

To solve the acoustic wave equation numerically, we adopt the staggered grids for the pressure and velocity variables. The configuration is shown in Figure SM1-left and we have used a uniform grid.

The major effort when discretizing the spatial derivative operator **??** is on the second term:

$$\Phi(x,t) = -\eta_x \int_0^t e^{-\alpha_x \tau}\partial_x c(x, t-\tau)d\tau. \tag{SM2.1}$$

With an increment of $\Delta t$, we have

$$\begin{aligned}
&\Phi(x, t+\Delta t)\\
=& -\eta^x \int_0^{t+\Delta t} e^{-\alpha^x\tau}\partial_x c(x, t+\Delta t-\tau)d\tau\\
=& -\eta^x \int_0^{t} e^{-\alpha^x\tau}\partial_x c(x, t+\Delta t-\tau)d\tau - \eta^x \int_t^{t+\Delta t} e^{-\alpha^x\tau}\partial_x c(x, t+\Delta t-\tau)d\tau\\
=& -\left(e^{-\alpha^x\Delta t}\right)\eta^x \int_0^{t} e^{-\alpha^x(t-\tau)}\partial_x c(x, \tau)d\tau - \eta^x \int_0^{\Delta t} e^{-\alpha^x\tau}\partial_x c(x, t+\Delta t-\tau)d\tau\\
\approx& \left(e^{-\alpha^x\Delta t}\right)\Phi(x,t) + \eta^x\left(\frac{e^{-\alpha^x\Delta t}-1}{\alpha^x}\right)\partial_x c(x, t+\Delta t).
\end{aligned} \tag{SM2.2}$$

Therefore, to compute $\partial_{\tilde{x}} c(x, t+\Delta t)$, we first compute $\partial_x c(x, t+\Delta t)$, update $\Phi(x, t+\Delta t)$ according to Equation (SM2.2), and then get $\partial_{\tilde{x}} c(x, t+\Delta t) = (1/\kappa^x)\partial_x c(x, t+\Delta t) + \Phi(x, t+\Delta t)$.

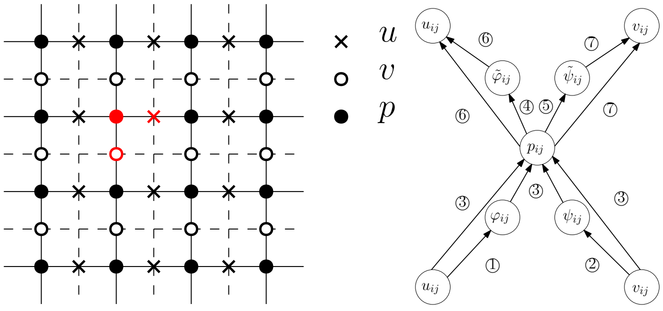


Fig. SM1: Left: Spatial staggered grid used in the discretization of the acoustic wave equation **??**. The red markers correspond to $u_{ij}$, $v_{ij}$ and $p_{ij}$ respectively. Right: Computation dependency graph for **??**.

We use $\delta_x$ and $\delta_y$ to denote the forward finite difference operators in $x$ axis and $y$ axis. For example the forth-order scheme reads

$$\begin{aligned}\delta_x c_{ij} &:= \frac{1}{24}c_{i-\frac{3}{2},j} - \frac{9}{8}c_{i-\frac{1}{2},j} + \frac{9}{8}c_{i+\frac{1}{2},j} - \frac{1}{24}c_{i+\frac{3}{2},j}\\ \delta_y c_{ij} &:= \frac{1}{24}c_{i,j-\frac{3}{2}} - \frac{9}{8}c_{i,j-\frac{1}{2}} + \frac{9}{8}c_{i,j+\frac{1}{2}} - \frac{1}{24}c_{i,j+\frac{3}{2}}\end{aligned} \tag{SM2.3}$$

Introducing the memory variables $\varphi_{ij}$, $\psi_{ij}$, $\tilde{\varphi}_{ij}$, $\tilde{\psi}_{ij}$, then the discretized acoustic wave equation with CPML boundary condition is

$$\begin{aligned}\varphi_{ij}^{n+\frac{1}{2}} &= \varphi_{ij}^{n-\frac{1}{2}} \exp\left(-\alpha_x^i \Delta t\right) + \eta_x^i \left(\frac{\exp\left(-\alpha_x^i \Delta t\right) - 1}{\alpha_x^i}\right)\frac{\delta_x u_{ij}^n}{\Delta x}\\ \psi_{ij}^{n+\frac{1}{2}} &= \psi_{ij}^{n-\frac{1}{2}} \exp\left(-\alpha_y^j \Delta t\right) + \eta_y^j \left(\frac{\exp\left(-\alpha_y^j \Delta t\right) - 1}{\alpha_y^j}\right)\frac{\delta_y v_{ij}^n}{\Delta y}\\ \frac{p_{ij}^{n+\frac{1}{2}} - p_{ij}^{n-\frac{1}{2}}}{\Delta t} &= K_{ij}\left(\frac{1}{\kappa_x^i}\frac{\delta_x u_{ij}^n}{\Delta x} + \varphi_{ij}^{n+\frac{1}{2}} + \frac{1}{\kappa_y^j}\frac{\delta_y v_{ij}^n}{\Delta y} + \psi_{ij}^{n+\frac{1}{2}}\right) + s_{ij}^n\\ \tilde{\varphi}_{ij}^{n+1} &= \tilde{\varphi}_{ij}^{n} \exp\left(-\tilde{\alpha}_x^i \Delta t\right) + \tilde{\eta}_x^i \left(\frac{\exp\left(-\tilde{\alpha}_x^i \Delta t\right) - 1}{\tilde{\alpha}_x^i}\right)\frac{\delta_x p_{i,j+\frac{1}{2}}^{n+\frac{1}{2}}}{\Delta x}\\ \tilde{\psi}_{ij}^{n+1} &= \tilde{\psi}_{ij}^{n} \exp\left(-\tilde{\alpha}_y^j \Delta t\right) + \tilde{\eta}_y^j \left(\frac{\exp\left(-\tilde{\alpha}_y^j \Delta t\right) - 1}{\tilde{\alpha}_y^j}\right)\frac{\delta_y p_{i+\frac{1}{2},j}^{n+\frac{1}{2}}}{\Delta y}\\ \rho_{ij}\frac{u_{ij}^{n+1} - u_{ij}^n}{\Delta t} &= \frac{1}{\kappa_x^i}\frac{\delta_x p_{i,j+\frac{1}{2}}^{n+\frac{1}{2}}}{\Delta x} + \tilde{\varphi}_{ij}^{n+1}\\ \rho_{ij}\frac{v_{ij}^{n+1} - v_{ij}^n}{\Delta t} &= \frac{1}{\kappa_y^j}\frac{\delta_y p_{i+\frac{1}{2},j}^{n+\frac{1}{2}}}{\Delta y} + \tilde{\psi}_{ij}^{n+1}\end{aligned} \tag{SM2.4}$$

that is, for every iteration, we perform the updates

$$\begin{bmatrix}\varphi^{n-\frac{1}{2}}\\ \psi^{n-\frac{1}{2}}\\ p^{n-\frac{1}{2}}\\ \tilde{\varphi}^n\\ \tilde{\psi}^n\\ u^n\\ v^n\end{bmatrix} \rightsquigarrow \begin{bmatrix}\varphi^{n+\frac{1}{2}}\\ \psi^{n+\frac{1}{2}}\\ p^{n+\frac{1}{2}}\\ \tilde{\varphi}^{n+1}\\ \tilde{\psi}^{n+1}\\ u^{n+1}\\ v^{n+1}\end{bmatrix} \tag{SM2.5}$$

The update is not necessarily sequential. Figure SM1-right shows the computation dependency of the forward propagation operator Equation (SM2.4).

The CFL stability condition for this system is [SM2, SM1]

$$\Delta t < \frac{\min(\Delta x, \Delta y)}{\max(v_{ij})\sqrt{2}}\left(\frac{9}{8} + \frac{1}{24}\right)^{-1}, \tag{SM2.6}$$

where $v_{ij} = \sqrt{K_{ij}/\rho_{ij}}$.

## REFERENCES

[SM1] R. W. Graves, *Simulating seismic wave propagation in 3d elastic media using staggered-grid finite differences*, Bulletin of the Seismological Society of America, 86 (1996), pp. 1091–1106.

[SM2] A. R. Levander, *Fourth-order finite-difference p-sv seismograms*, Geophysics, 53 (1988), pp. 1425–1436.
